# Supplementary material for: GDC- Generalized Distribution Calibration for Few-Shot Learning
Source: arXiv:2204.05230 source file (2022-04-11)
Supplement: Supplementary file 1 [file appendix.tex]

% This is samplepaper.tex, a sample chapter demonstrating the
% LLNCS macro package for Springer Computer Science proceedings;
% Version 2.21 of 2022/01/12
%
\documentclass[runningheads]{llncs}
%
\usepackage[T1]{fontenc}
\input{math_commands.tex}

% T1 fonts will be used to generate the final print and online PDFs,
% so please use T1 fonts in your manuscript whenever possible.
% Other font encondings may result in incorrect characters.
%
\usepackage{graphicx}
% Used for displaying a sample figure. If possible, figure files should
% be included in EPS format.
%
% If you use the hyperref package, please uncomment the following two lines
% to display URLs in blue roman font according to Springer's eBook style:
\usepackage{hyperref}
\usepackage{url}
\usepackage{algorithm}
\usepackage{algpseudocode}
\usepackage{multirow}

\usepackage{color}
\renewcommand\UrlFont{\color{blue}\rmfamily}


%
\begin{document}

\section*{Supplementary}
\appendix



\end{document}
